# Supplementary material for: Gaussian Universality of Perceptrons with Random Labels
Source: arXiv:2205.13303 source file (2023-03-02)
Supplement: Supplementary file 1 [file replica.tex]

\section{Appendix}
\label{appendix}
\subsection{Replica Analysis}

In this section, we provide a detailed derivation of the analytical results in sec. (\ref{section3}). The calculation is tackled by means of the replica method from statistical physics. 

\subsubsection{Boltzmann-Gibbs Formulation}
As we have seen in the main manuscript, the replica method allows to re-frame the learning problem in eq. (\ref{eq:optimization_w}) as a dynamical and exploratory process across the weight space. At equilibrium, we assume the weights to be distributed according to the Boltzmann-Gibbs measure, where the role of the Hamiltonian is actually played by the loss function defined on the dataset $\mathcal{D}$ in sec. (\ref{Model}):

\begin{align}
    \pi_{\beta}\left( \mathbf{w}, \mathcal{D} \right)  &= \frac{1}{\mathcal{Z}_{\beta}}\prod_{\mu = 1}^n e^{-\beta \ell\left(y_{\mu}, f_{\mathbf{w}}\left(\mathbf{x}_{\mu}\right) \right) }\prod_{i = 1}^p e^{ -\frac{\beta\lambda}{2} w^2_i}=\frac{P_{y}\left(Y|X,\mathbf{w} \right) P_w\left(\mathbf{w} \right)}{\mathcal{Z}_{\beta}} \notag\\
   &=\frac{1}{\mathcal{Z}_\beta} e^{-\beta\left( \sum_{\mu = 1}^n \ell\left(y_{\mu}, f_{\mathbf{w}}\left(\mathbf{x}_{\mu}\right) + \frac{\lambda}{2} \vert\vert \mathbf{w} \vert\vert_2^2\right) \right)}
\end{align}

with $X \in \mathbb{R}^{n\times p}$ being the matrix of all input data-points and $Y \in \mathbb{R}^n$ being the vector containing all the $n$ labels. The Boltzmann-Gibbs measure can thus be equivalently interpreted as the posterior of the Bayesian inference problem in eq. (\ref{eq:optimization_w}), whose likelihood and prior are defined by the two probability distributions $P_y\left( \cdot \right)$ and $P_w\left( \cdot \right)$ respectively. In the limit of zero temperature or, in other words, for $\beta \rightarrow \infty$, the Boltzmann-Gibbs distribution concentrates precisely on the minima of the training loss function, which are nothing but the solutions of the optimization problem in eq.(\ref{eq:optimization_w}). Re-framing a learning problem in terms of statistical physics does not seem to be a great advantage considering that sampling from the Boltzmann-Gibbs measure is known to be not feasible in the high-dimensional limit, i.e. $n,p \rightarrow \infty$ while $\alpha = p/n$ fixed. This is where the replica method comes into the game. As we have seen in the main manuscript, the replica trick allows us to compute the typical value over different realization of the dataset $\mathcal{D}$ of the free-energy density, namely:

\begin{equation}
\mathcal{F}_{\beta} = -\underset{p \rightarrow \infty}{\mbox{lim}}\frac{1}{p} \mathbb{E}_{\mathcal{D}}\mbox{log}\mathcal{Z}_{\beta}     
\end{equation}

From this quantity, all the other quantities of interest, including the training loss can be easily computed by following the replica recipe. In particular, the replica method allows us to compute the following parameters:

\begin{equation}
    Q_\star = \frac{\mathbf{\hat{w}}^t \Sigma \mathbf{\hat{w}}}{p} \hspace{10mm} M_\star = \frac{\mathbf{\hat{w}}^t \mathbf{\mu}}{p}
\end{equation}

with $\mathbf{\hat{w}}$ being the solution of the optimization problem in eq.(\ref{eq:optimization_w}) or, equivalently, the ground states of the Boltzmann-Gibbs measure $\pi_{\beta}$. As we will see, the training loss, which in principle is an high-dimensional quantity, can be easily expressed in terms of these simple scalar quantities $Q_\star$ and $M_\star$.

\subsubsection{Replica Calculation}
The replica calculation is based on the fact that, the free energy density in eq. (\ref{eq:free_energy_density-beta}) is a \emph{self-averaging} random variable, meaning that, in the thermodynamic limit its distribution is sharply peaked around its typical value over different realization of the training set. As we have seen in the main manuscript, the typical free-energy density can be computed by means of the replica method through the realization of $r \in \mathbb{N}$ distinct and independent copies of the same learning system:

\begin{equation}
\mathcal{F}_{\beta} =  -\underset{r\rightarrow 0^+}{\lim}\frac{d}{dr}\underset{p\rightarrow \infty}{\lim}\left[ \frac{\mathbb{E}_{\mathcal{D}} \mathcal{Z}^r_{\beta}\left(\mathcal{D}\right)}{p}  \right] 
\end{equation}

The averaged replicated partition function is therefore the starting point of the replica calculation. Re-writing it explicitly we have:

\begin{equation}
\mathbb{E}_{\mathcal{D}} \mathcal{Z}^r_{\beta}\left(\mathcal{D}\right) = \mathbb{E}_{\mathcal{D}} \left[\int \prod_{a = 1}^r d\mathbf{w}^a \prod_{a = 1}^r P_w\left( \mathbf{w}^a\right) \prod_{\mu = 1}^n \prod_{a = 1}^r P_y\left(y^{\mu}|\frac{\mathbf{x}_{\mu} \cdot \mathbf{w}^a}{\sqrt{p}} \right)\right]
\end{equation}

\paragraph{Average over the training dataset} The first step of the replica calculation recipe is the average over the training dataset. To this end, we first define the pre-activations as:
\begin{equation}
    h_a^{\mu} = \frac{\mathbf{x}_{\mu} \cdot \mathbf{w}^a}{\sqrt{p}}
\end{equation}

We then express this definition in terms of the Dirac-delta and its integral representation as:
\begin{equation}
    1 \propto \int \prod_{a = 1}^r\prod_{\mu = 1}^n  dh^{\mu}_a \ \delta\left( h_a^{\mu} -  \frac{\mathbf{x}_{\mu} \cdot \mathbf{w}^a}{\sqrt{p}}\right) = \int \prod_{a = 1}^r\prod_{\mu = 1}^n  \frac{dh^{\mu}_a d\hat{h}^{\mu}_a}{2\pi} \ \mbox{exp}\left(i\hat{h}_{a}^{\mu}\left( h_a^{\mu} -  \frac{\mathbf{x}_{\mu} \cdot \mathbf{w}^a}{\sqrt{p}}\right)\right)
\end{equation}

Finally we insert this factor one into the expression of the replicated partition function, thus getting:

\begin{equation}
\begin{split}
\mathbb{E}_{\mathcal{D}} \mathcal{Z}^r_{\beta}\left(\mathcal{D}\right) &= \int \prod_{a = 1}^r d\mathbf{w}^a \prod_{a = 1}^r P\left( \mathbf{w}^a\right) \prod_{\mu = 1}^n \prod_{a = 1}^r \frac{dh^{\mu}_a d\hat{h}^{\mu}_a}{2\pi} \mbox{exp}\left(i\sum_{a=1}^r\hat{h}_{\mu}^a h_{\mu}^a \right) \times\\
&\times \prod_{\mu = 1}^n \mathbb{E}_{y_\mu} \left[\prod_{a = 1}^r P_y\left(y_{\mu}|h_{\mu}^a \right)\mathbb{E}_{\mathbf{x}_\mu}\left[\mbox{exp}\left(-i\sum_{a = 1}^r\hat{h}_{\mu}^a \frac{\mathbf{x}_{\mu} \cdot \mathbf{w}^a}{\sqrt{p}}\right)\right]\right]
\end{split}
\end{equation}

In the high-dimensional limit, the average over the input data-points $\{ \mathbf{x}_{\mu}\}_{\mu = 1}^n$ can be performed by Taylor-expansion of the exponential up to the second order in $p$:

\begin{equation}
\begin{split}
    \mathbb{E}_{\mathbf{x}_\mu}\left[\mbox{exp}\left(-i\sum_{a = 1}^r\hat{h}_{\mu}^a \frac{\mathbf{x}_{\mu} \cdot \mathbf{w}^a}{\sqrt{p}}\right)\right] &= 1 -i\sum_{a = 1}^r\hat{h}_{\mu}^a \frac{\mathbb{E}_{\mathbf{x}_{\mu}}\left[\mathbf{x}_{\mu}\right] \cdot \mathbf{w}^a}{\sqrt{p}} - \frac{1}{2} \sum_{a,b = 1}^r \frac{\left(\mathbf{w^a}\right)^t  \mathbb{E}_{\mathbf{x}_{\mu}}\left[\mathbf{x}^t_{\mu}\mathbf{x}_{\mu}\right]\mathbf{w}^b}{p}\\
    & = \mbox{exp}\left( -i\sum_{a = 1}^r \frac{\mathbf{m} \cdot \mathbf{w}^a}{p}\hat{h}_{\mu}^a - \frac{1}{2} \sum_{a,b = 1}^r \frac{\left(\mathbf{w^a}\right)^t  \Sigma \mathbf{w}^b}{p}\hat{h}_{\mu}^a \hat{h}_{\mu}^b\right)
\end{split}
    \end{equation}

where we have defined $\mathbf{m}/\sqrt{p}$ as the mean of the input data-points and $\Sigma$ as the corresponding covariance matrix. Note that, while performing the average over the inputs we did not make any particular assumption on the input-data distribution except that it has to be characterized by a well-defined mean and covariance. This is for instance the case of the Gaussian Covariate model or the Gaussian Mixtures model defined in sec. (\ref{Model}) of the main manuscript. Having avergaed over the input data-points, the replicated partition function turns out to be given by:

\begin{equation}
\begin{split}
\mathbb{E}_{\mathcal{D}} \mathcal{Z}^r_{\beta}\left(\mathcal{D}\right) &= \int \prod_{a = 1}^r d\mathbf{w}^a \prod_{a = 1}^r P_w\left( \mathbf{w}^a\right) \prod_{\mu = 1}^n \prod_{a = 1}^r \frac{dh^{\mu}_a d\hat{h}^{\mu}_a}{2\pi} \mbox{exp}\left(i\sum_{a=1}^r\hat{h}_{\mu}^a h_{\mu}^a \right) \times\\
&\times \prod_{\mu = 1}^n \mathbb{E}_{y_\mu} \left[\prod_{a = 1}^r P_y\left(y_{\mu}|h_{\mu}^a \right)\mbox{exp}\left( -i\sum_{a = 1}^r \frac{\mathbf{m} \cdot \mathbf{w}^a}{p}\hat{h}_{\mu}^a - \frac{1}{2} \sum_{a,b = 1}^r \frac{\left(\mathbf{w}^a\right)^t  \Sigma \mathbf{w}^b}{p}\hat{h}_{\mu}^a \hat{h}_{\mu}^b\right)\right]
\end{split}
\end{equation}

\paragraph{Introduction of the overlap parameters.} As a direct consequence of the averaging process over the input data-points, the replicas are now interacting. To proceed further in the calculation and work in the direction of decoupling the different copies of the learning system, we can once again introduce the definition of the following overlap parameters:

\begin{equation}
    M^a = \frac{\mathbf{m} \cdot \mathbf{w}^a}{p} \hspace{15mm} Q^{ab} = \frac{\left(\mathbf{w}^a \right)^t \Sigma \mathbf{w}^b}{p} 
\end{equation}

by means of Dirac-deltas and their integral representation as:

\begin{equation}
\begin{split}
    1 &\propto \int \prod_{a = 1}^r  dM^a \prod_{a = 1}^r \delta\left( M^a -  \frac{\mathbf{m} \cdot \mathbf{w}^a}{p}\right) \prod_{a \leq b}  dQ^{ab} \prod_{a \leq b} \delta\left( Q^{ab} -  \frac{\left(\mathbf{w}^a \right)^t \Sigma \mathbf{w}^b}{p} \right)\\
    &= \int \prod_{a = 1}^r \frac{dM^a d\hat{M}^a}{2\pi} \ \mbox{exp}\left(i\sum_{a = 1}^r\hat{M}^{a}\left( M^a -  \frac{\mathbf{m} \cdot \mathbf{w}^a}{p}\right)\right)\int \prod_{a \leq b}^r \frac{dQ^{ab} d\hat{Q}^{ab}}{2\pi} \ \mbox{exp}\left(i\sum_{a = 1}^r\hat{Q}^{ab}\left( Q^{ab} -  \frac{\left(\mathbf{w}^a \right)^t \Sigma \mathbf{w}^b}{p}\right)\right)
\end{split}
\end{equation}

As before, we can insert this factor one into the expression of the replicated partition function, thus getting: 

\begin{equation}
\mathbb{E}_{\mathcal{D}} \mathcal{Z}^r_{\beta}\left(\mathcal{D}\right) = \int \prod_{a = 1}^r \frac{dM^a d\hat{M}^a}{2\pi} \int \prod_{a \leq b}^r \frac{dQ^{ab} d\hat{Q}^{ab}}{2\pi} \mbox{exp}\left(p \Psi_\beta^{(r)}\left( \{ M^a, \hat{M}^a \}_{a = 1}^r, \{Q^{ab}, \hat{Q}^{ab} \}_{a\leq b} \right) \right)\label{eq:replica_saddle_point_appendix} \end{equation}

with the potential $\Psi_\beta^{(r)}\left( \cdot \right)$ given by the sum of the following three terms:
\begin{equation}
\begin{split}
    &\psi = i\sum_{a = 1}^r \hat{M}^a M^a + i\sum_{a\leq b} \hat{Q}^{ab} Q^{ab}\\
    &\psi_w = \frac{1}{p}\mbox{log} \int \prod_{a = 1}^r d\mathbf{w}^a \prod_{a = 1}^r P_w\left( \mathbf{w}^a \right) \mbox{exp}\left(-i\sum_{a = 1}^r \hat{M}^a \mathbf{m}\cdot \mathbf{w}^a - i\sum_{a\leq b} \hat{Q}^{ab} \left( \mathbf{w}^a \right)^t \Sigma \mathbf{w}^b \right)\\
    &\psi_y = \alpha \mbox{log}\ \mathbb{E}_y \left[ \int \prod_{a = 1}^r \frac{dh^a d\hat{h}_a}{2\pi} \mbox{exp}\left(i\sum_{a = 1}^r \hat{h}_a h_a\right)  \prod_{a = 1}^r P_y\left(y|h_a \right) \mbox{exp}\left( -i\sum_{a = 1}^r \hat{h}_a M^a - \frac{1}{2}\sum_{a,b = 1}^r \hat{h}_a \hat{h}_b Q^{ab} \right)\right]
\end{split}\label{eq:replica_potentials_appendix}
\end{equation}

The term $\psi_w \left( \cdot \right)$ is often called prior channel or entropic potential because it encodes all the prior information of the weights of the learning model through the prior $P_w\left( \cdot \right)$, while $\psi_y\left( \cdot \right)$ is often called output channel or energetic potential because it incorporates all the information relative to both the labels and the training loss by mean of the likelihood $P_y\left( \cdot \right)$.
All the above steps have lead to express the averaged replicated function as a saddle-point integral with respect to the input dimension $p$. In the limit $r\rightarrow 0^+$ and $p\rightarrow\infty$, this directly leads to eq. (\ref{eq:saddle-point_integrals_before_replica_ansatz}) in the main manuscript. The drawback of this operation is that we have now to deal with $r$ interacting copies of the learning system. To proceed further into the calculation, we need to postulate a specific replica structure. In the following, we will thus investigate two possible assumptions: the so-called \emph{replica-symmetry} (RS) assumption and the so-called \emph{one-step replica symmetry breaking} (1-RSB) assumption.
\paragraph{Replica Symmetry} As shown in the main manuscript, since all replicas have been introduced independently from each other with no specific differences among them, it seems natural to assume that replicas should all play the same role. This inevitably leads to assume that the overlap paramaters and their hats counterparts should not depend on the specific replica index. In particular we assume:
\begin{equation}
\begin{split}
    Q^{ab}&=
    \begin{cases}
      R & \text{if}\ a = b \\
      Q & \text{otherwise}
    \end{cases} \hspace{15mm} -i\hat{Q}^{ab}=
    \begin{cases}
      -\frac{1}{2}\hat{R} & \text{if}\ a = b \\
      \hat{Q} & \text{otherwise}
    \end{cases}\\\\
M^a &= M \hspace{10mm} \forall a \hspace{22mm} -i\hat{M}^a = \hat{M} \\ 
\end{split}
\end{equation}
Applying this ansatz to eq. (\ref{eq:replica_saddle_point_appendix})-(\ref{eq:replica_potentials_appendix}), after some steps of algebra we then get the following expression for the three-terms of the $\Psi_{\beta}^{(r)} \left( \cdot \right)$ potential. Concerning the first term we have:

\begin{equation}
    \psi = -rM\hat{M} + \frac{r}{2}R\hat{R} - \frac{1}{2}r\left( r - 1\right) Q\hat{Q}
\end{equation}

Concerning the prior term we instead have:
\begin{equation}
    \psi_w = \frac{1}{p}\mbox{log} \int \prod_{a = 1}^r d\mathbf{w}^a \prod_{a = 1}^r P_w\left( \mathbf{w}^a \right) \mbox{exp}\left(\hat{M}\sum_{a = 1}^r \mathbf{m}\cdot \mathbf{w}^a - \frac{\hat{R}}{2}\sum_{a=1}^r \left( \mathbf{w}^a \right)^t \Sigma \mathbf{w}^a +\frac{\hat{Q}}{2} \sum_{a\leq b} \left( \mathbf{w}^a \right)^t \Sigma \mathbf{w}^b \right)
\end{equation}
In order to decouple the replicas, we can then apply the following Hubbard-Stratonovich transformation:
\begin{equation}
\mbox{exp}\left(\frac{\hat{Q}}{2} \sum_{a\leq b} \left( \mathbf{w}^a \right)^t \Sigma \mathbf{w}^b  \right) = \int \mathcal{D}\boldsymbol{\xi} \ \mbox{exp}\left(\sum_{a = 1}^r\left( \mathbf{w}^a \right)^t\left( \hat{Q}\Sigma \right)^{1/2} \boldsymbol{\xi}\right)
\end{equation}

with $\boldsymbol{\xi} \sim \mathcal{N}\left(0, \mathbf{I}_p \right)$. We can insert the Hubbard-Stratonovich transformation in the expression of the prior channel, which, having decoupled all the replicas, can be now factorized over the replica index: 
\begin{equation}
    \psi_w = \frac{1}{p}\mbox{log}\int \mathbb{E}_{\boldsymbol{\xi}} \left[ \int  d\mathbf{w} P_w\left( \mathbf{w} \right) \mbox{exp}\left(\hat{M} \mathbf{m}\cdot \mathbf{w}- \frac{\hat{R}}{2} \mathbf{w}^t \Sigma \mathbf{w} + \mathbf{w}^t\left( \hat{Q}\Sigma \right)^{1/2} \boldsymbol{\xi}\right)\right]^r
\end{equation}

Following the same steps, we can express the output channel in the same way as:
\begin{equation}
    \psi_y = \alpha \left[\mbox{log}\ \mathbb{E}_{y,\xi} \left[ \int \frac{dhd\hat{h}}{2\pi} P_y\left(y|h \right) \mbox{exp}\left( -\frac{1}{2} \left( R - Q \right)\hat{h}^2 + i \left( h + \sqrt{Q}\xi - M \right) \hat{h}\right) \right]\right]^r
\end{equation}
with $\xi \sim \mathcal{N}\left(0., 1. \right)$.However, in this case we are not yet done since we can here integrate the Gaussian integral over $\hat{h}$, thus getting:
\begin{equation}
    \psi_y = \alpha \left[\mbox{log}\ \mathbb{E}_{y,\xi} \left[ \int \frac{dh}{\sqrt{2\pi\left(R - Q \right)}} P_y\left(y|h \right) \mbox{exp}\left( - \frac{\left( h - \sqrt{Q}\xi - M \right)^2}{2\left( R - Q \right)}\right) \right]\right]^r
\end{equation}

At this point, we can combine these results and then take both the limit of $r \rightarrow 0^+$ and the limit of $p \rightarrow \infty$. This automatically allows to obtain the following free-energy density in the RS assumption:

\begin{equation}
\mathcal{F}_{\beta} =  -\underset{r\rightarrow 0^+}{\lim}\frac{d}{dr}\underset{p\rightarrow \infty}{\lim}\left[ \frac{\mathbb{E}_{\mathcal{D}} \mathcal{Z}^r_{\beta}\left(\mathcal{D}\right)}{p}  \right] = \underset{Q,R,M,\hat{Q},\hat{R},\hat{M}}{\mbox{extr}}\left[ \Psi_\beta^{(0)} \left(Q,R,M,\hat{Q},\hat{R},\hat{M} \right)\right] 
\label{eq:RS_free_energy_finite_beta}
\end{equation}

with the RS-potential $\Psi_\beta^{(0)}\left( \cdot \right)$ being given by the sum of the following three potentials:
\begin{equation}
\begin{split}
    &\psi = \frac{1}{2}R\hat{R} + \frac{1}{2}Q\hat{Q} - M\hat{M}\\
    &\psi_w = \underset{p\rightarrow\infty}{\lim} \frac{1}{p} \mathbb{E}_{\boldsymbol{\xi}}\left[ \mbox{log}\int d\mathbf{w} P_w\left( \mathbf{w} \right) \mbox{exp}\left(-\frac{1}{2}\mathbf{w}^t \left( \hat{R} + \hat{Q} \right)\Sigma \mathbf{w} + \mathbf{w}^t\left( \left(\hat{Q}\Sigma \right)^{1/2} \boldsymbol{\xi} + \hat{M}\mathbf{m}\right)\right)\right]\\
    & \psi_y = \alpha  \mathbb{E}_{y,\xi} \left[ \mbox{log} \int \frac{dh}{\sqrt{2\pi\left(R - Q \right)}}\mbox{exp}\left( - \frac{\left( h - \sqrt{Q}\xi - M \right)^2}{2\left( R - Q \right)}\right) P_y\left(y|h \right) \right]
\end{split}
\label{eq:RS_potentials_finite_beta}
\end{equation}

Indeed, in this limit, the only contribution to the saddle-point integrals in eq. (\ref{eq:replica_potentials_appendix})-(\ref{eq:replica_saddle_point_appendix}) comes from the extremizers of the replica symmetric potential $\Psi_\beta^{(0)}$.

\paragraph{One-step replica symmetry breaking} As pointed out in the main manuscript, the one-step replica symmetry breaking assumption aims to describe all those situations in which the space of solutions of the learning problem in eq. (\ref{eq:optimization_w}) breaks into more than one single ensemble of solutions. Because of that, in this case, it seems more reasonable to introduce one overlap parameters among replicas belonging to the same ensemble and another one among replicas belonging to different ensembles. We therefore assume:

\begin{equation}
\begin{split}
    Q^{ab}&=
    \begin{cases}
      R & \text{if}\ a = b \\
      Q_1 & \text{if}\ a \neq b \ \mbox{and} \ 0<\vert a - b \vert< x_0\\
      Q_0 &\mbox{otherwise}
    \end{cases} \hspace{15mm} -i\hat{Q}^{ab}=
    \begin{cases}
      -\frac{1}{2}\hat{R} & \text{if}\ a = b \\
      \hat{Q}_1 & \text{if}\ a \neq b \ \mbox{and} \ 0<\vert a - b \vert< x_0\\
      \hat{Q}_0 &\mbox{otherwise}
    \end{cases}\\\\
M^a &= M \hspace{10mm} \forall a \hspace{51mm} -i\hat{M}^a = \hat{M} \\ 
\end{split}
\end{equation}

In other words, the 1-RSB assumption leads to the following structure for the overlap matrix $O$ and its conjugate $\hat{O}$:
\begin{equation}
 O = \begin{pmatrix}
B & Q_0 \\
Q_0 & B
\end{pmatrix} \in \mathbb{R}^{r\times r} \hspace{30mm} \hat{O} = \begin{pmatrix}
\hat{B} & \hat{Q}_0 \\
\hat{Q}_0 & \hat{B}
\end{pmatrix} \in \mathbb{R}^{r\times r}
\end{equation}

with the block matrices $B$ and $\hat{B}$ given by:
\begin{equation}
\hspace{10mm}   B = \begin{pmatrix}
R & Q_1 & ... & Q_1 \\
Q_1 & R & ... & Q_1 \\
. & . & . & .\\
Q_1 & ... & R & Q_1 \\
Q_1 & ... & Q_1 & R
\end{pmatrix} \in \mathbb{R}^{x_0\times x_0} \hspace{22mm}B = \begin{pmatrix}
-\frac{1}{2}\hat{R} & Q_1 & ... & Q_1 \\
\hat{Q}_1 & -\frac{1}{2}\hat{R} & ... & \hat{Q}_1 \\
. & . & . & .\\
\hat{Q}_1 & ... & -\frac{1}{2}\hat{R} & \hat{Q}_1 \\
\hat{Q}_1 & ... & \hat{Q}_1 & -\frac{1}{2}\hat{R}
\end{pmatrix} \in \mathbb{R}^{x_0\times x_0}
\end{equation}

Gven the structure of the two matrices $O$ and $\hat{O}$, we can easily decompose in the sum of the three different matrices, as it follows:
\begin{equation}
\begin{split}
    O &= \left(R - Q_1\right) \mathbb{I}_{r\times r} + \left( Q_1 - Q_0 \right) \begin{pmatrix}
\mathbb{I}_{x_0 \times x_0} & 0 & ... & 0 \\
0 & \mathbb{I}_{x_0 \times x_0} & ... & 0 \\
. & . & . & .\\
0 & ... & \mathbb{I}_{x_0 \times x_0} & 0 \\
0 & ... & 0 & \mathbb{I}_{x_0 \times x_0}
\end{pmatrix}_{r\times r} + Q_0\mathbb{I}_{r\times r}\\\\
\hat{O} &= -\frac{1}{2}\left(\hat{R} + \hat{Q}_1\right) \mathbb{I}_{r\times r} + \left( \hat{Q}_1 - \hat{Q}_0 \right) \begin{pmatrix}
\mathbb{I}_{x_0 \times x_0} & 0 & ... & 0 \\
0 & \mathbb{I}_{x_0 \times x_0} & ... & 0 \\
. & . & . & .\\
0 & ... & \mathbb{I}_{x_0 \times x_0} & 0 \\
0 & ... & 0 & \mathbb{I}_{x_0 \times x_0}
\end{pmatrix}_{r\times r} + \hat{Q}_0\mathbb{I}_{r\times r}
\end{split}
\end{equation}

Applying this ansatz to eq. (\ref{eq:replica_saddle_point_appendix})-(\ref{eq:replica_potentials_appendix}), after some steps of algebra, we then get the following expression for the three-terms of the $\Psi_{\beta}^{(r)} \left( \cdot \right)$ potential. Concerning the first term we have:

\begin{equation}
    \psi = -rM\hat{M} + \frac{1}{2} R\hat{R} - \frac{r}{2}\left(x_0 - 1 \right)Q_1\hat{Q}_1 -\frac{r}{2}\left(r - x_0 \right)Q_0 \hat{Q}_0 
\end{equation}

Concerning the prior channel $\Psi_w\left(\cdot \right)$ we instead obtain:
\begin{equation}
\begin{split}
 \psi_w &= \frac{1}{p}\mbox{log} \int \prod_{a = 1}^r d\mathbf{w}^a \prod_{a = 1}^r P_w\left( \mathbf{w}^a\right)\mbox{exp}\left( \hat{M} \sum_{a = 1}^r \mathbf{m} \cdot \mathbf{w}^a -\frac{\hat{R} + \hat{Q_1}}{2} \sum_{a = 1}^r \left(\mathbf{w}^a\right)^t \Sigma \mathbf{w}^a\right)\times\\
&\times \mbox{exp}\left( \frac{\hat{Q}_0}{2} \sum_{a,b = 1}^r \left( \mathbf{w}^a \right)^t \Sigma \mathbf{w}^b + \frac{\hat{Q}_1 - \hat{Q}_0}{2} \sum_{k = 1}^{r/x_0} \sum_{a,b\in k} \left( \mathbf{w}^a \right)^t \Sigma \mathbf{w}^b\right)
\end{split}
\end{equation}

As in the replica symmetric ansatz, in order to decouple the replicas, we apply the two following Hubbard-Stratonovich transformations:
\begin{equation}
    \begin{split}
        &\mbox{exp}\left(\frac{\hat{Q}_0}{2} \sum_{a,b = 1}^r \left( \mathbf{w}^a \right)^t \Sigma \mathbf{w}^b \right) = \mathbb{E}_{\boldsymbol{\xi}_0}\left[ \mbox{exp}\left(  \sum_{a = 1}^r \left( \mathbf{w}^a \right)^t \left( \hat{Q}_0 \Sigma \right)^{1/2}\boldsymbol{\xi}_0 \right)\right]\\
        &\mbox{exp}\left( \frac{\hat{Q}_1 - \hat{Q}_0}{2} \sum_{k = 1}^{r/x_0} \sum_{a,b\in k} \left( \mathbf{w}^a \right)^t \Sigma \mathbf{w}^b \right) = \prod_{k = 1}^{r/x_0} \mathbb{E}_{\boldsymbol{\xi}_1^k}\left[ \mbox{exp}\left(  \sum_{a \in k} \left( \mathbf{w}^a \right)^t \left( \left(\hat{Q}_1 - \hat{Q}_0\right) \Sigma \right)^{1/2}\boldsymbol{\xi}_1^k \right)\right]
    \end{split}
\end{equation}

with $\mathbf{\xi}_0, \mathbf{\xi}^k_1 \sim \mathcal{N}\left(0, \mathbf{I}_p\right)$. Having decoupled the different copies of the learning system, we can now factorize over the replica index, thus getting:

\begin{equation}
\begin{split}
 \psi_w &= \frac{1}{p} \mbox{log} \mathbb{E}_{\boldsymbol{\xi}_0}\left[ \mathbb{E}_{\boldsymbol{\xi}_1} \left[ \int d\mathbf{w} P_w\left( \mathbf{w}\right)\mbox{exp}\left( -\frac{1}{2} \mathbf{w}^t \left( \hat{R} + \hat{Q}_1 \right) \Sigma \mathbf{w}  \right) \right. \right. \times\\
 &\left. \left. \times \mbox{exp}\left(\mathbf{w}^t \left( \left(\left(\hat{Q}_1 - \hat{Q}_0 \right)\Sigma\right)^{1/2} + \left( \hat{Q}_0 \Sigma \right)^{1/2} \boldsymbol{\xi}_0 + \hat{M}\mathbf{m}\right) \right)\right]^{x_0}\right]^{r/x_0}
 \end{split}
\end{equation}

The same steps can be applied for the output channel $\Psi_y$, and, by further solving the Gaussian integral over $\hat{h}$, we then get:

\begin{equation}
    \psi_y = \alpha\mathbb{E}_{y,\xi_0} \mbox{log}\ \left[ \mathbb{E}_{\xi_1} \left[\int \frac{dh}{\sqrt{2\pi\left( R - Q_1 \right)}} \mbox{exp}\left(-\frac{\left( h - \sqrt{Q_0}\xi_0 -\sqrt{Q_1 - Q_0} \xi_1 \right)^2}{2\left( R - Q_1 \right)}\right)P_y\left( y|h\right) \right]^{x_0} \right]^{r/x_0}
\end{equation}

At this point, we can combine these results and then take both the limit of $r \rightarrow 0^+$ and the limit of $p \rightarrow \infty$. This automatically allows to obtain the following free-energy density in the 1-RSB assumption:

\begin{equation}
\mathcal{F}_{\beta} =  -\underset{r\rightarrow 0^+}{\lim}\frac{d}{dr}\underset{p\rightarrow \infty}{\lim}\left[ \frac{\mathbb{E}_{\mathcal{D}} \mathcal{Z}^r_{\beta}\left(\mathcal{D}\right)}{p}  \right] = \underset{Q_0,Q_1,R,M,\hat{Q}_0,\hat{Q}_1,\hat{R},\hat{M}}{\mbox{extr}}\left[ \Psi_\beta^{(0)} \left(Q_0,Q_1,R,M,\hat{Q}_0,\hat{Q}_1,\hat{R},\hat{M}\right)\right] 
\end{equation}

with the 1RSB-potential $\Psi_\beta^{(0)}\left( \cdot \right)$ being given by the sum of the following three potentials:
\begin{equation}
\begin{split}
    &\psi = \frac{1}{2}R\hat{R} - \frac{1}{2}\left(x_0 - 1 \right)Q_1\hat{Q}_1 + \frac{1}{2}x_0 Q_0 \hat{Q}_0 - M\hat{M}\\
    &\psi_w = \underset{p\rightarrow \infty}{\lim} \frac{1}{p x_0} \mathbb{E}_{\boldsymbol{\xi}_0} \mbox{log} \mathbb{E}_{\boldsymbol{\xi}_1} \left[ \int d\mathbf{w} P_w\left( \mathbf{w}\right)\mbox{exp}\left( -\frac{1}{2} \mathbf{w}^t \left( \hat{R} + \hat{Q}_1 \right) \Sigma \mathbf{w}  \right) \right. \times\\
    &\hspace{8mm}\left. \times \mbox{exp}\left(\mathbf{w}^t \left( \left(\left(\hat{Q}_1 - \hat{Q}_0 \right)\Sigma\right)^{1/2} + \left( \hat{Q}_0 \Sigma \right)^{1/2} \boldsymbol{\xi}_0 + \hat{M}\mathbf{m}\right) \right)\right]^{x_0}\\
    & \psi_y = \frac{\alpha}{x_0} \mathbb{E}_{y,\xi_0} \mbox{log} \mathbb{E}_{\xi_1} \left[ \int \frac{dh}{\sqrt{2\pi\left( R - Q_1 \right)}} \mbox{exp}\left(-\frac{\left( h - \sqrt{Q_0}\xi_0 -\sqrt{Q_1 - Q_0} \xi_1 \right)^2}{2\left( R - Q_1 \right)}\right)P_y\left( y|h\right) \right]^{x_0}
\end{split}
\end{equation}

Indeed, in this limit, the only contribution to the saddle-point integrals in eq. (\ref{eq:replica_potentials_appendix})-(\ref{eq:replica_saddle_point_appendix}) comes from the extremizers of the 1-RSB potential $\Psi_\beta^{(0)}$.

\subsubsection{Gaussian Prior}
As we have pointed out in the main manuscript, the learning problem we are interested in is linear classification with random labels and $l_2$-regularization. In the context of Bayesian inference, the $l_2$-regularization plays the role of a Gaussian prior on the learning weights. In this section, we will thus evaluate the free-energy density in the specific case of Gaussian priors, namely:
\begin{equation}
    P_w\left(\mathbf{w} \right) = \frac{1}{\left(2\pi\right)^{p/2}} \mbox{exp}\left(-\frac{1}{2}\beta \lambda \vert\vert \mathbf{w}\vert \vert_2^2 \right)
    \label{eq:Gaussian_Prior}
\end{equation}

\paragraph{Replica Symmetry}
Given the free-energy density in eq. (\ref{eq:RS_free_energy_finite_beta})-(\ref{eq:RS_potentials_finite_beta}), we can see that the entropic potential is the only one depending on the prior distribution. When evaluated on the Gaussian prior in eq. (\ref{eq:Gaussian_Prior}), the prior channel acquires the following form: 

\begin{equation}
    \psi_w = \underset{p\rightarrow\infty}{\lim} \frac{1}{p} \mathbb{E}_{\boldsymbol{\xi}}\left[ \mbox{log}\int d\mathbf{w} \ \mbox{exp}\left(-\frac{1}{2}\mathbf{w}^t \left(\beta\lambda\mathbb{I}_{p\times p}+\hat{V}\Sigma\right) \mathbf{w} + \mathbf{w}^t\left( \left(\hat{Q}\Sigma \right)^{1/2} \boldsymbol{\xi} + \hat{M}\mathbf{m}\right)\right)\right]
\end{equation}

where we have defined $\hat{V} = \hat{R} + \hat{Q}$. With the choice of a Gaussian prior, the integral over the learning weights can be easily solved as it is nothing but a standard Gaussian integral, providing the following expression for the entropic potential evaluated on Gaussian priors:

\begin{equation}
\begin{split}
   \psi_w &= -\underset{p \rightarrow \infty}{\mbox{lim}}\frac{1}{2p} \mbox{tr} \ \mbox{log}\left( \beta \lambda \mathbb{I}_{p\times p} + \hat{V} \Sigma \right) +\\ &+\underset{p \rightarrow \infty}{\mbox{lim}}\frac{1}{2p} \mathbb{E}_{\boldsymbol{\xi}} \left[ \left(\left( \hat{Q}\Sigma\right)^{1/2} \boldsymbol{\xi} + \hat{M}\mathbf{m}\right)^t\left( \beta \lambda \mathbb{I}_{p\times p} + \hat{V} \Sigma \right)^{-1}\left(\left( \hat{Q}\Sigma\right)^{1/2} \boldsymbol{\xi} + \hat{M} \mathbf{m}\right) \right]
 \end{split}
\end{equation}

where we have used the property of determinants, that is the logarithm of the determinant of a given matrix corresponds to the trace of the logarithm of the same matrix. By finally computing the Gaussian integral over $\boldsymbol{\xi}$, we finally get:

\begin{equation}
\begin{split}
   \psi_w &= -\underset{p \rightarrow \infty}{\mbox{lim}}\frac{1}{2p} \mbox{tr} \ \mbox{log}\left( \beta \lambda \mathbb{I}_{p\times p} +\hat{V}\Sigma \right) + \underset{p \rightarrow \infty}{\mbox{lim}}\frac{1}{2p} \mbox{tr} \left( \left( \beta \lambda \mathbb{I}_{p\times p} + \hat{V} \Sigma \right)^{-1}\hat{Q}\Sigma  \right) +\\
   &+ \underset{p\rightarrow \infty}{\lim} \frac{1}{2p} \left(\hat{M}\mathbf{m} \right)^t \left( \beta\lambda \mathbb{I}_{p\times p} + \hat{V}\Sigma  \right)^{-1}\left(\hat{M}\mathbf{m} \right)
 \end{split}
\end{equation}

The resulting free-energy density under the RS assumption for Gaussian prior is then given by:

\begin{equation}
\mathcal{F}_{\beta} = \underset{Q,V,M,\hat{Q},\hat{V},\hat{M}}{\mbox{extr}}\left[ \Psi_\beta^{(0)} \left(Q,V,M,\hat{Q},\hat{V},\hat{M} \right)\right] 
\label{eq:RS_free_energy_finite_beta_gp}
\end{equation}

with the RS-potential $\Psi_\beta^{(0)}\left( \cdot \right)$ evaluated on Gaussian priors given by the sum of the following three potentials:
\begin{equation}
\begin{split}
    &\psi = \frac{1}{2}\left(V + Q \right)( \hat{V} - \hat{Q}) + \frac{1}{2}Q\hat{Q} - M\hat{M}\\
    &\psi_w = -\underset{p \rightarrow \infty}{\mbox{lim}}\frac{1}{2p} \mbox{tr} \ \mbox{log}\left( \beta \lambda \mathbb{I}_{p\times p} + \hat{V} \Sigma \right) + \underset{p \rightarrow \infty}{\mbox{lim}}\frac{1}{2p} \mbox{tr} \left( \left( \beta \lambda \mathbb{I}_{p\times p} + \hat{V} \Sigma \right)^{-1}\hat{Q}\Sigma  \right)+\\
    &\hspace{9mm}+\underset{p \rightarrow \infty}{\mbox{lim}}\frac{1}{2p} \underset{p\rightarrow \infty}{\lim} \frac{1}{2p} \left(\hat{M}\mathbf{m} \right)^t \left(\beta\lambda \mathbb{I}_{p\times p} + \hat{V}\Sigma  \right)^{-1}\left(\hat{M}\mathbf{m} \right)\\
    & \psi_y = \alpha \mathbb{E}_{y,\xi} \left[\ \mbox{log} \int \frac{dh}{\sqrt{2\pi V}}\mbox{exp}\left( - \frac{\left( h - \sqrt{Q}\xi - M \right)^2}{2V}\right) P_y\left(y|h \right) \right]
\end{split}
\label{eq:RS_potentials_finite_beta}
\end{equation}

where we have defined $V = R - Q$.
\paragraph{Replica Symmetry Breaking} The prior channel under the one-step replica symmetry assumption, when evaluated on Gaussian priors, is given by the following expression:
\begin{equation}
\begin{split}
    &\psi_w = \underset{p\rightarrow \infty}{\lim} \frac{1}{p x_0} \mathbb{E}_{\boldsymbol{\xi}_0} \mbox{log} \mathbb{E}_{\boldsymbol{\xi}_1} \left[ \int d\mathbf{w} \ \mbox{exp}\left( -\frac{1}{2} \mathbf{w}^t \left( \beta \lambda \mathbb{I}_{p\times p} + \hat{V}_1 \Sigma\right) \mathbf{w}  \right) \right. \times\\
    &\hspace{8mm}\left. \times \mbox{exp}\left(\mathbf{w}^t \left( \left(\left(\hat{Q}_1 - \hat{Q}_0 \right)\Sigma\right)^{1/2}\boldsymbol{\xi}_1 + \left( \hat{Q}_0 \Sigma \right)^{1/2} \boldsymbol{\xi}_0 + \hat{M}\mathbf{m}\right) \right)\right]^{x_0}
\end{split}
\end{equation}

Where we have defined $\hat{V} = \hat{R} + \hat{Q}_1$. The integral over $\mathbf{w}$ can be easily solved being nothing but a standard Gaussian integral, thus getting the following expression for the prior channel $\Psi_w \left( \cdot \right)$:

\begin{equation}
    \begin{split}
        \psi_w &= - \underset{p \rightarrow \infty}{\lim} \frac{1}{2p} \mbox{tr}\ \mbox{log}\left(\beta \lambda \mathbb{I}_{p\times p} + \hat{V}_1 \Sigma \right) + \\
        & + \underset{p \rightarrow \infty}{\lim} \frac{1}{p x_0} \mathbb{E}_{\boldsymbol{\xi}_0}\mbox{log} \left[ \mathbb{E}_{\boldsymbol{\xi}_1}\left[\mbox{exp}\left(\frac{x_0}{2}\left( \left(\left(\hat{Q}_1 - \hat{Q}_0 \right)\Sigma\right)^{1/2} \boldsymbol{\xi}_1 + \left( \hat{Q}_0 \Sigma \right)^{1/2} \boldsymbol{\xi}_0 + \hat{M}\mathbf{m}\right)^t \right)\times \right. \right.\\
        &\left.\left.\times \mbox{exp}\left( \left( \beta \lambda \mathbb{I}_{p\times p} + \hat{V}_1 \Sigma\right)^{-1}  \left( \left(\left(\hat{Q}_1 - \hat{Q}_0 \right)\Sigma\right)^{1/2}\boldsymbol{\xi}_1 + \left( \hat{Q}_0 \Sigma \right)^{1/2} \boldsymbol{\xi}_0 + \hat{M}\mathbf{m}\right)\right)\right]\right]
    \end{split}
\end{equation}

The remaining integrals over $\boldsymbol{\xi}_0$ and  $\boldsymbol{\xi}_1$ are standard Gaussian integrals too. They can thus be directly solved, leading to the following expression for the prior channel: 

\begin{equation}
\begin{split}
\psi_w &=  -\underset{p \rightarrow \infty}{\lim}\frac{1}{2p} \mbox{tr} \ \mbox{log}\left( \beta \lambda \mathbb{I}_{p\times p} +\hat{V}_1 \Sigma \right) + \underset{p \rightarrow \infty}{\mbox{lim}}\frac{1}{2p} \mbox{tr} \left( \left( \beta \lambda \mathbb{I}_{p\times p} + \hat{V}_1 \Sigma \right)^{-1}\hat{Q}_0\Sigma  \right) +\\
&+\underset{p\rightarrow \infty}{\lim} \frac{1}{2p} \left(\hat{M}\mathbf{m} \right)^t \left( \beta\lambda \mathbb{I}_{p\times p} + \hat{V}_1\Sigma  \right)^{-1}\left(\hat{M}\mathbf{m} \right)+\\
& - \underset{p \rightarrow \infty}{\lim}\frac{1}{2p x_0} \mbox{tr}\ \mbox{log} \left( \mathbb{I}_{p\times p} -x_0 \left(\left(\hat{Q}_1 - \hat{Q}_0 \right) \Sigma \right)^{1/2} \left( \beta \lambda \mathbb{I}_{p\times p} + \hat{V}_1 \Sigma \right)^{-1}\left(\left(\hat{Q}_1 - \hat{Q}_0 \right) \Sigma \right)^{1/2} \right) +  \underset{p\rightarrow \infty}{\lim} \frac{x_0}{2p} \hat{Q}_0 \left( \hat{Q}_1 - \hat{Q}_0 \right) \times \\
& \times \mbox{tr}\left(
  \left( \beta \lambda \mathbb{I}_{p\times p} + \hat{V}_1 \Sigma \right)^{-2} \left( \mathbb{I}_{p\times p} -x_0 \left(\left(\hat{Q}_1 - \hat{Q}_0 \right) \Sigma \right)^{1/2} \left( \beta \lambda \mathbb{I}_{p\times p} + \hat{V}_1 \Sigma \right)^{-1}\left(\left(\hat{Q}_1 - \hat{Q}_0 \right) \Sigma \right)^{1/2} \right)\right)^{-1} +\\
& - \underset{p \rightarrow \infty}{\lim}\frac{x_0}{2p} \left( \hat{M} \mathbf{m} \right)^t \left( \left( \hat{Q}_1 - \hat{Q}_0 \right) \Sigma \right)^{1/2} \left( \beta \lambda \mathbb{I}_{p\times p} + \hat{V}_1 \Sigma \right)^{-1}\times \\
&\times \left( \mathbb{I}_{p\times p} -x_0 \left(\left(\hat{Q}_1 - \hat{Q}_0 \right) \Sigma \right)^{1/2} \left( \beta \lambda \mathbb{I}_{p\times p} + \hat{V}_1 \Sigma \right)^{-1}\left(\left(\hat{Q}_1 - \hat{Q}_0 \right) \Sigma \right)^{1/2} \right)^{-1}\times\\
&\times \left( \left( \hat{Q}_1 - \hat{Q}_0 \right) \Sigma \right)^{1/2} \left( \beta \lambda \mathbf{I} + \hat{V}_1 \Sigma \right)^{-1} \hat{M} \mathbf{m}
  \end{split}
\end{equation}

The resulting free-energy density under the RS assumption for Gaussian prior is then given by:

\begin{equation}
\mathcal{F}_{\beta} =  \underset{Q_0,Q_1,V_1,M,\hat{Q}_0,\hat{Q}_1,\hat{V}_1,\hat{M}}{\mbox{extr}}\left[ \Psi_\beta^{(0)} \left(Q_0,Q_1,V_1,M,\hat{Q}_0,\hat{V}_1,\hat{R},\hat{M}\right)\right] 
\end{equation}

with the 1RSB-potential $\Psi_\beta^{(0)}\left( \cdot \right)$ being given by the sum of the following three potentials:
\begin{equation}
\begin{split}
&\psi = \frac{1}{2}\left(V_1 +Q_1\right)\left( \hat{V}_1 - \hat{Q}_1\right) - \frac{1}{2}\left(x_0 - 1 \right)Q_1\hat{Q}_1 + \frac{1}{2}x_0 Q_0 \hat{Q}_0 - M\hat{M}\\
& \psi_w =  -\underset{p \rightarrow \infty}{\lim}\frac{1}{2p} \mbox{tr} \ \mbox{log}\left( \beta \lambda \mathbb{I}_{p\times p} +\hat{V}_1 \Sigma \right) + \underset{p \rightarrow \infty}{\mbox{lim}}\frac{1}{2p} \mbox{tr} \left( \left( \beta \lambda \mathbb{I}_{p\times p} + \hat{V}_1 \Sigma \right)^{-1}\hat{Q}_0\Sigma  \right) +\\
&+\underset{p\rightarrow \infty}{\lim} \frac{1}{2p} \left(\hat{M}\mathbf{m} \right)^t \left( \beta\lambda \mathbb{I}_{p\times p} + \hat{V}_1\Sigma  \right)^{-1}\left(\hat{M}\mathbf{m} \right)+\\
& - \underset{p \rightarrow \infty}{\lim}\frac{1}{2p x_0} \mbox{tr}\ \mbox{log} \left( \mathbb{I}_{p\times p} -x_0 \left(\left(\hat{Q}_1 - \hat{Q}_0 \right) \Sigma \right)^{1/2} \left( \beta \lambda \mathbb{I}_{p\times p} + \hat{V}_1 \Sigma \right)^{-1}\left(\left(\hat{Q}_1 - \hat{Q}_0 \right) \Sigma \right)^{1/2} \right) +  \underset{p\rightarrow \infty}{\lim} \frac{x_0}{2p} \hat{Q}_0 \left( \hat{Q}_1 - \hat{Q}_0 \right) \times \\
& \times \mbox{tr}\left(
  \left( \beta \lambda \mathbb{I}_{p\times p} + \hat{V}_1 \Sigma \right)^{-2} \left( \mathbb{I}_{p\times p} -x_0 \left(\left(\hat{Q}_1 - \hat{Q}_0 \right) \Sigma \right)^{1/2} \left( \beta \lambda \mathbb{I}_{p\times p} + \hat{V}_1 \Sigma \right)^{-1}\left(\left(\hat{Q}_1 - \hat{Q}_0 \right) \Sigma \right)^{1/2} \right)\right)^{-1} +\\
& - \underset{p \rightarrow \infty}{\lim}\frac{x_0}{2p} \left( \hat{M} \mathbf{m} \right)^t \left( \left( \hat{Q}_1 - \hat{Q}_0 \right) \Sigma \right)^{1/2} \left( \beta \lambda \mathbb{I}_{p\times p} + \hat{V}_1 \Sigma \right)^{-1}\times \\
&\times \left( \mathbb{I}_{p\times p} -x_0 \left(\left(\hat{Q}_1 - \hat{Q}_0 \right) \Sigma \right)^{1/2} \left( \beta \lambda \mathbb{I}_{p\times p} + \hat{V}_1 \Sigma \right)^{-1}\left(\left(\hat{Q}_1 - \hat{Q}_0 \right) \Sigma \right)^{1/2} \right)^{-1}\times\\
&\times \left( \left( \hat{Q}_1 - \hat{Q}_0 \right) \Sigma \right)^{1/2} \left( \beta \lambda \mathbf{I} + \hat{V}_1 \Sigma \right)^{-1} \hat{M} \mathbf{m}\\
& \psi_y = \frac{\alpha}{x_0} \ \mathbb{E}_{y,\xi_0} \mbox{log} \mathbb{E}_{\xi_1} \left[ \int \frac{dh}{\sqrt{2\pi\left( R - Q_1 \right)}} \mbox{exp}\left(-\frac{\left( h - \sqrt{Q_0}\xi_0 -\sqrt{Q_1 - Q_0} \xi_1 \right)^2}{2\left( R - Q_1 \right)}\right)P_y\left( y|h\right) \right]^{x_0}
\end{split}
\end{equation}

where we have defined $V_1 = R - Q_1$.
\subsubsection{Zero Temperature Limit}
The solutions of the optimization problem in eq. (\ref{eq:optimization_w}) correspond to the minima of the loss function, namely those weight configurations with the highest statistical significance in the zero-temperature limit. With the purpose of dealing with optimization problems, we therefore need to further take the zero-temperature limit of the replica equations in both replica symmetry and one-step replica symmetry breaking scenarios. 

\paragraph{Replica Symmetry} In the limit of $\beta \rightarrow \infty$, the overlap parameters obey the following scaling with respect to $\beta$:

\begin{equation}
\begin{split}
    Q &\sim O\left( 1 \right) \hspace{10mm} \hat{Q} \sim O\left( \beta^{-2}\right)\\
    V &\sim O\left( \beta \right) \hspace{10mm} \hat{V} \sim O\left( \beta^{-1}\right)\\
    M &\sim O\left( 1 \right) \hspace{10mm} \hat{M} \sim O\left( \beta^{-1}\right)\\
    x_0 &\sim O\left( \beta \right)
\end{split}\label{eq:beta_scaling}
\end{equation}

Applying the above scaling in $\beta$ for $\psi$ and $\psi_w$ is quite straightforward since it only requires the identification of the leading terms in $\beta$ and to neglect all the remaining once. This operation leads to the following results for the two potentials: 

\begin{equation}
\begin{split}
    &\psi = \underset{\beta \rightarrow \infty}{\lim}\frac{\psi}{\beta} = \frac{1}{2}\left(V\hat{Q} - \hat{V}Q \right) - M\hat{M}\\
    &\psi_w =\underset{\beta \rightarrow \infty}{\lim} \frac{\psi}{\beta} = \underset{p \rightarrow \infty}{\mbox{lim}}\frac{1}{2p} \underset{p\rightarrow \infty}{\lim} \frac{1}{2p} \left(\hat{M}\mathbf{m} \right)^t \left(\lambda \mathbb{I}_{p\times p} + \hat{V}\Sigma  \right)^{-1}\left(\hat{M}\mathbf{m} \right)+ \underset{p \rightarrow \infty}{\mbox{lim}}\frac{1}{2p} \mbox{tr} \left( \left( \lambda \mathbb{I}_{p\times p} + \hat{V} \Sigma \right)^{-1}\hat{Q}\Sigma  \right)
\end{split}
\label{eq:RS_potentials_finite_beta}
\end{equation}

Concerning the energetic potential, in order to detect the leading order in $\beta$ we first need to re-write the output channel in terms of the Boltzamnn-Gibbs measure:
\begin{equation}
\begin{split}
     \psi_y &= \alpha  \mathbb{E}_{y,\xi}\mbox{log} \left[ \int \frac{dh}{\sqrt{2\pi V}}\mbox{exp}\left( - \frac{\left( h - \sqrt{Q}\xi - M \right)^2 - \beta \ell\left( y, h\right)}{2V}\right) \right]\\
     & = \alpha  \mathbb{E}_{y,\xi}\mbox{log} \left[ \int \frac{dh}{\sqrt{2\pi V}}\mbox{exp}\left( -\beta \frac{\left( h - \sqrt{Q}\xi - M \right)^2 - \ell\left( y, h\right)}{2V}\right) \right]
\end{split}
\label{eq:RS_potentials_finite_beta}
\end{equation}

where in the last equality we have applied the scaling in (\ref{eq:beta_scaling}) for $V$. In the limit of $\beta \rightarrow \infty$, the dominant contribution to the $h$-integral is the one maximizing the argument of the exponential function. Because of that, in this limit, the energetic potential can be written as it follows:
\begin{equation}
    \psi_y = \underset{\beta \rightarrow \infty}{\lim}\frac{\psi_y}{\beta} = \alpha  \mathbb{E}_{y,\xi} \left[ \frac{\left( \eta - \omega \right)^2 - \ell\left( y, \eta\right)}{2V} \right]\label{eq:psi_y_zero_temperature}
\end{equation}

where we have defined $\omega = \sqrt{Q}\xi - M$ and $\eta$ being the extremizer of the argument of the exponential function:

\begin{equation}
    \eta = \underset{h \in \mathbb{R}}{\mbox{argmin}} \left[\frac{\left(h - \omega\right)^2}{2V_1} + \ell\left(y, h \right)\right]
    \label{eq:eta}
\end{equation}

By collecting all the different terms we finally get eq. (\ref{eq:free-energy}) with the potentials $\psi$, $\psi_w$ and $\psi_y$ defined as in the main manuscript.
\paragraph{Replica Symmetry Breaking} In the limit of $\beta \rightarrow \infty$, the overlap parameters obey the following scaling with respect to $\beta$:

\begin{equation}
\begin{split}
    Q_1 &\sim O\left( 1 \right) \hspace{10mm} \hat{Q}_1 \sim O\left( \beta^{-2}\right)\\
    Q_0 &\sim O\left( 1 \right) \hspace{10mm} \hat{Q}_0 \sim O\left( \beta^{-2}\right)\\
    V &\sim O\left( \beta \right) \hspace{10mm} \hat{V} \sim O\left( \beta^{-1}\right)\\
    M &\sim O\left( 1 \right) \hspace{10mm} \hat{M} \sim O\left( \beta^{-1}\right)\\
    x_0 &\sim O\left( \beta \right)
\end{split}\label{eq:beta_scaling}
\end{equation}

As in the RS assumption, applying the above scaling in $\beta$ for $\psi$ and $\psi_w$ is quite straightforward since it only requires the identification of the leading terms in $\beta$ and to neglect all the remaining once. This operation leads to the following results for the two potentials: 

\begin{equation}
\begin{split}
&\psi = \underset{\beta \rightarrow \infty}{\lim} \frac{1}{\beta} \psi= -\frac{1}{2}\left(V_1\hat{Q}_1 - \hat{V}_1Q_1 + x_0 \left( Q_1\hat{Q}_1 - Q_0\hat{Q}_0 \right)\right) - M\hat{M}\\
& \psi_w = \underset{\beta \rightarrow \infty}{\lim} \frac{1}{\beta} \psi_w = \underset{p \rightarrow \infty}{\mbox{lim}}\frac{1}{2p} \mbox{tr} \left( \left(  \lambda \mathbb{I}_{p\times p} + \hat{V}_1 \Sigma \right)^{-1}\hat{Q}_0\Sigma  \right) +\underset{p\rightarrow \infty}{\lim} \frac{1}{2p} \left(\hat{M}\mathbf{m} \right)^t \left( \lambda \mathbb{I}_{p\times p} + \hat{V}_1\Sigma  \right)^{-1}\left(\hat{M}\mathbf{m} \right)+\\
& +  \underset{p\rightarrow \infty}{\lim} \frac{x_0}{2p} \hat{Q}_0 \left( \hat{Q}_1 - \hat{Q}_0 \right) \times \\
& \times \mbox{tr}\left(
  \left( \lambda \mathbb{I}_{p\times p} + \hat{V}_1 \Sigma \right)^{-2} \left( \mathbb{I}_{p\times p} -x_0 \left(\left(\hat{Q}_1 - \hat{Q}_0 \right) \Sigma \right)^{1/2} \left(  \lambda \mathbb{I}_{p\times p} + \hat{V}_1 \Sigma \right)^{-1}\left(\left(\hat{Q}_1 - \hat{Q}_0 \right) \Sigma \right)^{1/2} \right)\right)^{-1} +\\
& - \underset{p \rightarrow \infty}{\lim}\frac{x_0}{2p} \left( \hat{M} \mathbf{m} \right)^t \left( \left( \hat{Q}_1 - \hat{Q}_0 \right) \Sigma \right)^{1/2} \left( \beta \lambda \mathbb{I}_{p\times p} + \hat{V}_1 \Sigma \right)^{-1}\times \\
&\times \left( \mathbb{I}_{p\times p} -x_0 \left(\left(\hat{Q}_1 - \hat{Q}_0 \right) \Sigma \right)^{1/2} \left( \beta \lambda \mathbb{I}_{p\times p} + \hat{V}_1 \Sigma \right)^{-1}\left(\left(\hat{Q}_1 - \hat{Q}_0 \right) \Sigma \right)^{1/2} \right)^{-1}\times\\
&\times \left( \left( \hat{Q}_1 - \hat{Q}_0 \right) \Sigma \right)^{1/2} \left( \beta \lambda \mathbb{I}_{p\times p} + \hat{V}_1 \Sigma \right)^{-1} \left(\hat{M} \mathbf{m}\right)\\
\end{split}
\end{equation}

For what concerns the energetic potential, we can apply exactly the same reasoning seen for replica symmetry in the previous paragraph. This will lead to the following expression for the energetic potential:

\begin{equation}
\psi_y = \underset{\beta \rightarrow \infty}{\lim} \frac{1}{\beta} =\frac{\alpha}{x_0}\mathbb{E}_{y,\xi_0} \left[\mbox{log} \ \mathbb{E}_{\xi_1}\left[ \mbox{exp}\left(-x_0\left( \frac{\left(\eta_1 - \omega_1\right)^2}{2V_1} + \ell\left(y, \eta_1 \right) \right)\right)\right]\right]
\end{equation}

By combining the expression of the three potentials in the zero-temperature limit, we finally get the free-energy density of eq.(\ref{eq:free-energy_1rsb}) in the main manuscript. 

\subsubsection{Saddle Point equations under Replica Symmetry Assumption} The extremum operation in eq. (\ref{eq:free-energy}) requires the differentiation of the corresponding free-energy density with respect to both the overlap parameters and their conjugates. This leads to a set of coupled saddle-point equations, which for the overlap parameters are given by:  
\begin{equation}
   \begin{split}
       Q & = -2\frac{\partial \psi_w}{\partial\hat{V}} = -\frac{\hat{M}^2}{p} \mathbf{m}^t \left( \lambda \mathbb{I}_{p\times p} + \hat{V}\Sigma \right)^{-2} \Sigma \mathbf{m} + \mbox{tr}\left( \hat{Q}\Sigma \left( \lambda \mathbb{I}_{p\times p + \hat{V}\Sigma} \right)^{-2} \Sigma \right)\\
       V & = 2\frac{\partial\psi_w}{\partial \hat{Q}} = \mbox{tr}\left(\Sigma \left( \lambda\mathbb{I}_{p\times p} + \hat{V}\Sigma \right)^{-1} \right) \\
       M &=\frac{\partial \psi_w}{\partial \hat{M}} = \frac{\hat{M}}{p} \mathbf{m}^t \left(\lambda \mathbb{I}_{p\times p} + \hat{V}\Sigma \right)^{-1} \mathbf{m}
   \end{split} 
\end{equation}

The saddle-point equations involving the conjugate overlap parameters, do actually depend on the specific choice of the training loss, since they involve the energetic potential through partial derivatives with respect to the overlap parameters. In this work we have derived those relative to the square and the hinge loss.
\paragraph{Square Loss} In the specific case of the square loss function, the one-sample loss $\ell\left(y, h \right)$ in eq. (\ref{eq:eta}), is given by:
\begin{equation}
\ell\left( y, h\right) = \frac{1}{2} \left(y - h \right)^2    
\end{equation}

By plugging the square one-sample loss in eq. (\ref{eq:eta}), we then get the following expression for the extremizer $\eta$:
\begin{equation}
    \eta = \frac{\omega + yV}{1+V}
\end{equation}

If we evaluate the energetic potential of eq. (\ref{eq:psi_y_zero_temperature}) in $\eta$, we can then easily solve the Gaussian integral over $\xi$ and the one over the uniformly distributed $y$. The integration will give as the following expression for the output channel:
\begin{equation}
    \psi_y = -\frac{\alpha}{2}\left(  \frac{1+Q+M^2}{1+V}\right)
\end{equation}

From this simple expression of the output channel, we can straightforwardly determine the saddle-point equations for the overlap parameters:

\begin{equation}
    \begin{split}
        \hat{Q} &= 2\frac{\partial \psi_y}{\partial V} = \frac{1+Q+M^2}{\left( 1 + V\right)^2}\\
        \hat{V} &= -2\frac{\partial \psi_y}{\partial Q} = \frac{1}{1+V}\\
        \hat{M} &= \frac{\partial \psi_y}{\partial M} = \frac{M}{1+V}
    \end{split}
\end{equation}

\paragraph{Hinge Loss} In the specific case of the square loss function, the one-sample loss $\ell\left(y, h \right)$ in eq. (\ref{eq:eta}), is given by:
\begin{equation}
\ell\left( y, h\right) = \mbox{max} \left(0, 1- yh \right)    
\end{equation}

By plugging the square one-sample loss in eq. (\ref{eq:eta}), we then get the following expression for the extremizer $\eta$ by considering all the possible cases required by the max non-linearity:

\begin{equation}
    \eta = \begin{cases}
      \omega \ \text{if} \ y\omega \geq 1 \\
      y \ \text{if} \ 1-V \geq y\omega \leq 1 \\
      \omega + yV\ \text{if} \ y\omega \leq 1-V \\
    \end{cases}
\end{equation}

If we evaluate the energetic potential of eq. (\ref{eq:psi_y_zero_temperature}) in $\eta$, we can then easily solve the Gaussian integral over $\xi$ and the one over the uniformly distributed $y$. The integration will give as the following expression for the output channel:
\begin{equation}
    \psi_y = \psi^+_{y,1} + \psi^+_{y,2} + \psi^-_{y,1} + \psi^-_{y,2}  
\end{equation}

where the above four terms given by:
\begin{equation}
    \begin{split}
    \psi_{y,1}^{\pm} &= -\frac{\sqrt{Q}\left( 1 \mp M \right)}{4\sqrt{2\pi}V} \mbox{exp}\left( -\frac{\left( 1 \mp M\right)^2}{2Q}\right) + \frac{\sqrt{Q}\left( 1 \mp M + V\right)}{4\sqrt{2\pi}V} \mbox{exp}\left( -\frac{\left( 1 \mp M - V\right)^2}{2Q}\right)+\\
    &-\frac{Q + \left( 1 \mp M\right)^2}{8V} \left( \mbox{erf}\left(\frac{1\mp M}{\sqrt{2Q}} - \frac{1\mp M-V}{\sqrt{2Q}} \right) \right)\\
    \psi_{y,2}^{\pm} &= -\frac{1}{2}\left( \sqrt{\frac{Q}{2\pi}} \mbox{exp} \left( - \frac{\left( 1 - \mp M -V \right)^2}{2Q}\right) + \frac{1-M-V/2}{2}\left(1 + \mbox{erf}\left(\frac{1 \mp M -V}{\sqrt{2Q}} \right)\right) \right)
    \end{split}
\end{equation}

From this expression of the output channel, we can then determine the corresponding saddle-point equations for the overlap parameters:
\begin{itemize}
    \item saddle-point equation for $\hat{Q}$: 
    \begin{equation}
        \hat{Q} = 2\frac{\partial \psi_y}{\partial V} = -\partial_V \left[ \psi^+_{y,1} + \psi^+_{y,2} + \psi^-_{y,1} + \psi^-_{y,2} \right]
\end{equation}

where the partial derivatives are given by:
\begin{equation}
\begin{split}
    \partial_V \psi^{\pm}_{y,1} &= \frac{\left(\frac{V^3}{\sqrt{Q}} + \sqrt{Q}\left(1 \mp M + V \right) \right) \mbox{exp}\left(-\frac{\left( 1 \mp M - V\right)^2}{2Q} \right) - \sqrt{Q}\left(1\mp M \right) \mbox{exp}\left(-\frac{\left( 1 \mp M \right)^2}{2Q} \right)}{2\sqrt{2\pi} V^2} +\\
    & - \frac{1}{4V^2} \left( \left( 1 \mp M\right)^2 + Q \right)\left( \mbox{erf}\left( \frac{1\mp M}{\sqrt{2Q}}\right) - \mbox{erf}\left(\frac{1\mp M-V}{\sqrt{2Q}} \right) \right)\\
    \partial_V \psi^{\pm}_{y,2} &= -\frac{V}{2\sqrt{2\pi Q}} \mbox{exp}\left(-\frac{\left( 1 \mp M -V\right)^2}{2Q} \right) - \frac{1}{4}\left( 1 + \mbox{erf}\left(\frac{1\mp M-V}{\sqrt{2Q}} \right) \right) 
\end{split}
\end{equation}
\item saddle-point equation for $\hat{V}$:
\begin{equation}
        \hat{V} =- 2\frac{\partial \psi_y}{\partial Q} = \partial_Q \left[ \psi^+_{y,1} + \psi^+_{y,2} + \psi^-_{y,1} + \psi^-_{y,2} \right]
\end{equation}
where the partial derivatives are given by:
\begin{equation}
    \begin{split}
    \partial_Q \psi^{\pm}_{y,1} &= -\frac{\left(2Q - \left( 1 \mp M -V\right)V \right)}{4\sqrt{2\pi}Q^{3/2}}\mbox{exp}\left(-\frac{\left(1 \mp M -V \right)^2}{2Q} \right) +\frac{1}{4V} \left( \mbox{erf}\left(\frac{1\mp M}{\sqrt{2Q}} \right) - \mbox{erf}\left(\frac{1 \mp M-V}{\sqrt{2Q}} \right)  \right)\\
    \partial_Q \psi^{\pm}_{y,2} &= \frac{2Q - \left(1 \mp M-V \right)V}{4\sqrt{2\pi}Q^{3/2}} \mbox{exp}\left(-\frac{\left(1\mp M-V \right)^2}{2Q} \right)
    \end{split}
\end{equation}
\item saddle-point equation for $\hat{M}$:
\begin{equation}
        \hat{M} =- 2\frac{\partial \psi_y}{\partial M} =-\frac{1}{2} \partial_M \left[ \psi^+_{y,1} + \psi^+_{y,2} + \psi^-_{y,1} + \psi^-_{y,2} \right]
\end{equation}
where the partial derivatives are given by:
\begin{equation}
    \begin{split}
        \partial_M \psi^{\pm}_{y,1} &= \mp \frac{Q}{\sqrt{2\pi Q}V}\mbox{exp}\left(-\frac{\left( 1\mp M\right)^2}{2Q} \right) + \frac{\left(2Q + V^2 \right)}{2\sqrt{2\pi Q}V} \mbox{exp}\left(-\frac{\left( 1\mp M\right)\left(1\mp M -2V \right)+V^2}{2Q} \right) +\\
        &\pm \frac{1\mp M}{2V}\left(\mbox{erf}\left(\frac{1\mp M-V}{\sqrt{2Q}} \right) - \mbox{erf}\left(\frac{1\mp M}{\sqrt{2Q}} \right) \right)\\
        \partial_M \psi^{\pm}_{y,1} &= \mp \frac{V}{2\sqrt{2\pi Q}}\mbox{exp}\left(-\frac{\left( 1 \mp M -V\right)^2}{2Q} - \frac{1}{2} \left( 1 + \mbox{erf}\left(\frac{1\mp M-V}{\sqrt{2Q}} \right)\right)\right)
    \end{split}
\end{equation}

\end{itemize}

\subsection{Technical Details of the Simulations}
