# Supplementary material for: Gaussian Universality of Perceptrons with Random Labels
Source: arXiv:2205.13303 source file (2023-03-02)
Supplement: Supplementary file 2 [file universality.tex]

\section{Mathematical arguments towards universality of Gaussian Mixtures}\label{app:gaussian_universality}

We work in a setting slightly more general than the main text; the minimization problem we consider is of the form
\begin{equation}\label{eq:def_min_problem}
 \widehat\cR_n^*(\bm X, \bm y) = \inf_{\bm \Theta \in \cS_p^k} \frac1n\sum_{\mu=1}^n \ell(\bm \Theta^\top \bm x_\mu, y_\mu) + r(\bm\Theta),
\end{equation}
where the $\bm x_\mu \in \dR^p$ are input vectors, $y_\mu\in \dR$ are one-dimensional labels, and $\cS_p$ is a compact subset of $\dR^p$. We assume that the loss $\ell$ only depends on the $x_\mu$ through $k$ one-dimensional projections $\bm\theta_1^\top \bm x_\mu, \dots, \bm \theta_k^\top \bm x_\mu$, and we work in the so-called proportional high-dimensional limit, where $n, p$ go to infinity with
\[\frac np \to \alpha > 0, \]
while $k$ stays fixed.

Throughout this section, $\norm{}$ will denote the spectral norm of a matrix, while $\norm{}_q$ for $q > 0$ will refer to the element-wise $q$-norms. For a subgaussian random variable $Y$, its sub-gaussian norm $\norm{Y}_{\psi_2}$ is defined as
\[ \norm{Y}_{\psi_2} = \inf \Set*{t > 0 \given \E*{\exp\left(\frac{Y^2}{t^2}\right)} \leq 2}. \]

\addtocontents{toc}{\protect\setcounter{tocdepth}{1}}
\subsection{State of the art}
\addtocontents{toc}{\protect\setcounter{tocdepth}{2}}

There have been many recent progress on Gaussian-type low-dimensional CLT and universality recently \cite{goldt2020gaussian,hu_universality_2021,montanari2022universality}. We shall leverage on these results to prove our first theorem.

In particular, the starting point for our mathematical proof will use the recent result of \cite{montanari2022universality} which we shall now review. Consider the minimization problem
\eqref{eq:def_min_problem}, with $(\bm x_\mu, y_\mu)$ i.i.d random variables; the goal is to replace the $\bm x_\mu$ by their Gaussian equivalent model
\begin{equation} 
    \bm g_\mu \overset{i.i.d}{\sim} \cN(\bm 0, \bm \Sigma) \qquad \text{where}\qquad \bm \Sigma = \E*{\bm x\bm x^\top}.
\end{equation}
We make the following assumptions:

\begin{assump}[Loss and regularization]\label{assump:loss}
    The loss function $\ell : \dR^{k+1} \to \dR$ is nonnegative and Lipschitz, and the regularization function $r : \dR^{p\times k} \to \dR$ is locally Lipschitz, with constants independent from $p$.
\end{assump}

\begin{assump}[Labels]\label{assump:labels}
    The $y_\mu$ are generated according to
    \begin{equation}\label{eq:label_definition_montanari}
    y_\mu = \eta(\bm \Theta^* \bm x_\mu, \eps_\mu),
    \end{equation}
    where $\eta : \dR^{k^*+1}\to \dR$ is a Lipschitz function, $\bm \Theta^* \in \cS_p^{k^*}$, and the $\eps_\mu$ are i.i.d subgaussian random variables with
    \[ \norm{\eps_\mu}_{\psi_2} \leq M \]
    for some constant $M > 0$.
\end{assump}

\begin{assump}[Concentration on the directions of $\cS_p$]\label{assump:concentration}
    We have
    \begin{equation}\label{eq:isotropy_montanari}
    \sup_{\bm \theta \in \cS_p, \norm{\bm \theta}_2 \leq 1} \norm{\bm \theta^\top \bm x}_{\psi_2} \leq M \qquand \sup_{\bm \theta \in \cS_p, \norm{\bm \theta}_2 \leq 1} \norm{\bm \Sigma \bm \theta}_{2} \leq M,
    \end{equation}
    for some constant $M > 0$.
\end{assump}

\begin{assump}[One-dimensional CLT]\label{assump:clt}
    For any bounded Lipschitz function $\varphi: \dR \to \dR$,
    \begin{equation}
        \lim_{p\to \infty} \sup_{\bm \theta\in\cS_p} \E*{\left\lvert\phi(\bm \theta^\top \bm x) - \phi(\bm \theta^\top \bm g)\right\rvert} = 0.
    \end{equation}
\end{assump}

Building on those assumptions, \cite{montanari2022universality} prove the following:
\begin{theorem}[Theorem 1. in \cite{montanari2022universality}] \label{thm:montanari_universality}
Suppose that Assumptions \ref{assump:loss}-\ref{assump:clt} hold. Then, for any bounded Lipschitz function $\Phi: \dR \to \dR$, we have
\[\lim_{n, p \to \infty} \left| \E*{\Phi\left(\widehat\cR_n^*(\bm X, \bm y(\bm X))\right)} - \E*{\Phi\left(\widehat\cR_n^*(\bm G, \bm y(\bm G))\right)} \right| = 0\]

In particular, for any $\rho \in \dR$,
\[ \widehat\cR_n^*(\bm X, \bm y(\bm X)) \overset{\dP}{\longrightarrow} \rho \quad \text{if and only if} \quad \widehat\cR_n^*(\bm G, \bm y(\bm G)) \overset{\dP}{\longrightarrow} \rho \]
\end{theorem}

\subsection{Sketch of proof of Theorem \ref{thm:montanari_universality}, adapted from \cite{montanari2022universality}}

\paragraph{Free energy approximation} Define the discretized free energy
\begin{equation}
    f_{\epsilon, \beta}(\bm X) = \frac1{n\beta}\sum_{\bm\Theta\in\cN_\epsilon^k} \exp\left( -\beta\,  \widehat\cR_n(\bm\Theta ; \bm X, \bm y(\bm X) ) \right),
\end{equation}
where $\widehat\cR_n(\bm\Theta ; \bm X, \bm y(\bm X) )$ is the quantity minimized in \eqref{eq:def_min_problem}, and $\cN_\epsilon$ is a minimal $\epsilon$-net of $\cS_p$. Using classical arguments from both the theory of $\epsilon$-nets and statistical physics, the authors show that
\begin{equation}\label{eq:free_energy_approx}
    \left|f_{\epsilon, \beta}(\bm X) - \widehat\cR_n(\bm\Theta ; \bm X, \bm y(\bm X) \right| \leq C_1(\epsilon) + \frac{C_2(\epsilon)}{\beta},
\end{equation}
and the same inequality holds for $\bm G$. Since $C_1, C_2$ do not depend on $n, p$, it is possible to choose first $\epsilon$, then $\beta$ so that the RHS of \eqref{eq:free_energy_approx} is as small as desired, and keep them fixed throughout the rest of the proof. We can therefore focus on studying the free energy approximation $f_{\epsilon, \beta}$ throughout the rest of the proof.

\paragraph{Interpolation path}
For any $0 \leq t \leq \pi/2$, define
\[ \bm U_t = \cos(t)\bm X + \sin(t) \bm G\]
Then $\bm U_t$ is a smooth interpolation path with independent columns, ranging from $\bm U_0 = \bm X$ to $\bm U_{\pi/2} = \bm G$. We can write, for any differentiable function $\psi$,
\[ \left|\E*{\psi(f_{\epsilon, \beta}(\bm X))} - \E*{\psi(f_{\epsilon, \beta}(\bm G))} \right| \leq \int_0^{\pi/2} \left|\E*{\frac{d \psi(f_{\epsilon, \beta}(\bm U_t)))}{dt}}\right|  dt,\]
and by the dominated convergence theorem it suffices to show that the integrand converges to $0$ for any $t$. The chain rule gives
\[ \frac{d \psi(f_{\epsilon, \beta}(\bm U_t)))}{dt} = \psi'(f_{\epsilon, \beta}(\bm U_t)))\left( \sum_{\mu=1}^n \left(\frac{d\bm u_{t, \mu}}{dt}\right)^\top \nabla_{\bm u_{t, \mu}} f_{\epsilon, \beta}(\bm U_t) \right), \]

and the dependency in $\psi$ can be easily controlled. Since all columns of $\bm U_t$ are i.i.d, we are left with showing
\begin{equation}\label{eq:interp_universality}
    \lim_{n, p \to \infty} n \dE_{(1)}\left[\left(\frac{d\bm u_{t, 1}}{dt}\right)^\top \nabla_{\bm u_{t, 1}} f_{\epsilon, \beta}(\bm U_t)\right] = 0 \quad \text{a.s.},
\end{equation}
where $\dE_{(1)}$ denotes the expectation with respect to $(\bm x_1, \bm g_1, \eps_1)$.

\paragraph{Showing \eqref{eq:interp_universality}}

Imagine for a moment that $\bm x_1$ is Gaussian; then $\bm u_{t, 1}$ and $d\bm u_{t, 1}/dt$ are also jointly Gaussian, and we have
\begin{align*}
\E*{\left(\frac{d\bm u_{t, 1}}{dt}\right)^\top \bm u_{t, 1}} &= \E*{(-\sin(t)\bm x_1 + \cos(t)\bm g_1)^\top (\cos(t)\bm x_1 + \sin(t)\bm g_1)} \\
&= 0,
\end{align*}
since $x_1$ and $g_1$ have the same covariance by definition. Therefore, they are independent, and we have
\begin{align*}
    \dE_{(1)}\left[\left(\frac{d\bm u_{t, 1}}{dt}\right)^\top \nabla_{\bm u_{t, 1}} f_{\epsilon, \beta}(\bm U_t)\right] = \dE_{(1)}\left[\left(\frac{d\bm u_{t, 1}}{dt}\right)\right]^\top \dE_{(1)}\left[\nabla_{\bm u_{t, 1}} f_{\epsilon, \beta}(\bm U_t)\right] = 0.
\end{align*}
On the other hand, it is possible to show that $\bm x_1$ only appears in \eqref{eq:interp_universality} through scalar products with $\bm \Theta$ or $\bm \Theta^*$. As a result, we can leverage Assumption $\ref{assump:clt}$ to replace $\bm x_1$ by a Gaussian vector $\bm w$ independent from $\bm g_1$ as $p \to \infty$. Then, the reasoning above can be repeated with $\bm w$ and $\bm g_1$ to conclude the proof.

\subsection{Proof of Theorem \ref{thm:main_gaussian_universality}}
In order to prove our theorem \ref{thm:main_gaussian_universality}, we now aim to adapt the proof from \cite{montanari2022universality} to the case where the distribution of $x$ can be a {\it mixture} of several other distributions, each with different mean and covariance. For a discrete set $\cC = \{1, \dots, K\}$, we consider a family of distributions $(\nu_c)_{c\in \cC}$ on $\dR^p$, with means and covariances
\[ \bm \mu_c = \dE_{\bm z\sim \nu_c}[\bm z] \qquand \bm \Sigma_c = \dE_{\bm z\sim \nu_c}[\bm z \bm z^\top] \]
Given a type assignment $\sigma: [n] \to \cC$, each sample $x_\mu$ is then drawn independently from $\nu_{\sigma(\mu)}$. The equivalent Gaussian model is straightforward: we simply take
\[ \bm g_i \sim \cN(\bm \mu_{\sigma(\mu)}, \bm \Sigma_{\sigma(\mu)}), \]
independently from each other. An important special case of this setting is when $\sigma$ is itself random, independently from the $\bm x_i$ and $\bm g_i$: the law of $\bm g_i$ is then a so-called Gaussian Mixture Model.

The assumptions of Theorem \ref{thm:montanari_universality} are modified as follows:
\begin{enumerate}
    \item Assumption \ref{assump:loss} is unchanged,
    \item We relax \eqref{eq:label_definition_montanari} in Assumption \ref{assump:labels} into 
    \[ y_i = \eta_{\sigma(i)}(\bm \Theta^* \bm x_i, \eps_i), \]
    for a family $(\eta_c)_{c\in \cC}$ of Lipschitz functions. This allows in particular to incorporate classification problems in our setting, at no cost in the proof complexity.
    \item We impose in Assumption \ref{assump:concentration} the stronger condition
    \begin{equation}\label{eq:app:gaussian_subgaussian}
        \sup_{\bm \theta \in \cS_p, \norm{\bm \theta}_2 \leq 1} \norm{\bm \theta^\top \bm g}_{\psi_2} \leq M,
    \end{equation} 
    which is a consequence of \eqref{eq:isotropy_montanari} when $g$ has zero-mean. This is in practice an additional condition on the means $\bm \mu_c$; indeed, \eqref{eq:app:gaussian_subgaussian} is equivalent to
    \begin{equation}
        \sup_{\bm \theta \in \cS_p, \norm{\bm \theta}_2 \leq 1} \langle \bm \mu_c, \bm \theta \rangle \leq M' \quand \sup_{\bm \theta \in \cS_p, \norm{\bm \theta}_2 \leq 1} \norm{\bm \Sigma_c\, \bm \theta}_{2} \leq M',
    \end{equation}
    for some different constant $M'$.
    \item We suppose that Assumptions \ref{assump:concentration} and \ref{assump:clt} hold for any possible distribution $\nu_c$ for $c \in \cC$ and its associated Gaussian equivalent model.
\end{enumerate}

Our result is then an extension of Theorem \ref{thm:montanari_universality} for mixtures:

\begin{reptheorem}{thm:main_gaussian_universality}
Suppose that the modified above assumptions hold. Then, for any bounded Lipschitz function $\Phi: \dR \to \dR$, we have
\[\lim_{n, p \to \infty} \left| \E*{\Phi\left(\widehat\cR_n^*(\bm X, \bm y(\bm X))\right)} - \E*{\Phi\left(\widehat\cR_n^*(\bm G, \bm y(\bm G))\right)} \right| = 0\]

In particular, for any $\rho \in \dR$,
\[ \widehat\cR_n^*(\bm X, \bm y(\bm X)) \overset{\dP}{\longrightarrow} \rho \quad \text{if and only if} \quad \widehat\cR_n^*(\bm G, \bm y(\bm G)) \overset{\dP}{\longrightarrow} \rho \]
\end{reptheorem}

We now go through the proof of the previous section, highlighting the important changes.

\paragraph{Free energy approximation} This section goes basically unchanged; the approximation between $\widehat\cR_n^*(\bm X, \bm y(\bm X))$ and $f_{\epsilon, \beta}(\bm X)$ relies on Lipschitz arguments and concentration bounds on the $\bm x_i$ and $\bm g_i$, which are satisfied by our modification of Assumption \ref{assump:concentration}.

\paragraph{Interpolation path} Recall that the important property of $\bm U_t$ is that
\begin{equation}\label{eq:ut_constant_norm}
\E*{\left(\frac{d\bm U_t}{dt}\right)^\top \bm U_t} = 0.
\end{equation}
To this end, we set
\[ \bm u_{t, \mu} = \bm \mu_{\sigma(\mu)} + \cos(t)(\bm x_\mu - \bm \mu_{\sigma(\mu)}) + \sin(t)(\bm g_\mu - \bm \mu_{\sigma(\mu)}), \]
and it is easy to check that \eqref{eq:ut_constant_norm} is satisfied.

Another problem is that the columns of $\bm U_t$ are not i.i.d anymore, so we have to control
\begin{equation}\label{eq:interp_non_iid}
    \frac 1n \sum_{\mu=1}^n \left| \dE_{(\mu)}\left[\left(\frac{d\bm u_{t, \mu}}{dt}\right)^\top \nabla_{\bm u_{t, \mu}} f_{\epsilon, \beta}(\bm U_t)\right] \right|,
\end{equation}
where this time $\dE_{(\mu)}$ is the expectation w.r.t $(\bm x_\mu, \bm g_\mu, \eps_\mu)$. However, \eqref{eq:interp_non_iid} is a weighted average over all values of $\sigma(\mu)$, and since $\cC$ is finite is suffices to show \eqref{eq:interp_universality} for any value of $\sigma(1)$.

\paragraph{Showing \eqref{eq:interp_universality}} This section again relies on concentration properties of the $\bm x_i$ and $\bm g_i$, as well as Assumption \ref{assump:clt}. The arguments thus translate directly from \cite{montanari2022universality}.

\subsection{One-dimensional gaussian approximation}

Although Theorem \ref{thm:montanari_universality} is a powerful result, it still relies on very strong assumptions. In particular, given a distribution $\nu$ for the inputs $\bm x_i$, characterizing the set of vectors $\bm \theta$ such that Assumption \ref{assump:clt} holds is in general a difficult task.

\paragraph{Rigorous results} When the entries of $\bm x$ are i.i.d subgaussian, a classical application of the Lindeberg method \citep{lindeberg_1922_eine} shows that Assumptions \ref{assump:concentration} and \ref{assump:clt} are satisfied with
\[ \cS_p = \Set*{\bm \theta \in \dR^p \given \norm{\bm \theta}_\infty  = o_p(1)}. \]
More recently, this result (often used under the name ``Gaussian Equivalence Theorem'') was extended to general feature models with approximate orthogonality constraints \citep{hu_universality_2021,goldt2020gaussian}, for the same choice of $\cS_p$. \cite{montanari2022universality} also provides a central limit theorem result for the Neural Tangent Kernel of \citep{jacot2018neural}, for a more convoluted parameter set $\cS_p$. While these papers provide a strong basis for the one-dimensional CLT, those rigorous results only concern (so far) a very restricted set of distributions.

\paragraph{Concentration of the norm} Another, more informal line of work originating from \cite{seddik_2020_random}, argues that most distributions found in the real world satisfy some form of the central limit theorem. The starting point of this analysis is the following theorem, adapted from \cite{bobkov_concentration_2003}:
\begin{theorem}[Corollary 2.5 from \cite{bobkov_concentration_2003}]\label{thm:almost_everywhere_clt}
Let $\bm x \in\dR^p$ be a random variable, with $\E*{\bm x\bm x^\top} = \bm I_p$, and $\eta_p$ the smallest positive number such that
\begin{equation}\label{eq:norm_concentration}
\Pb*{\left| \frac{\norm{\bm x}_2}{\sqrt{p}} - 1 \right| \geq \eta_p} \leq \eta_p.
\end{equation}
Then for any $\delta > 0$, there exists a subset $\cS_p$ of the $p$-sphere $\dS^{p-1}$ of measure at least $4p^{3/8}e^{-c p\delta^4}$, such that
\[ \sup_{\bm \theta\in \cS_p} \sup_{t\in \dR} \left|\Pb{\bm \theta^\top \bm x \geq t} - \Phi(t) \right| \leq \delta + 4\eta_p,\]
where $\Phi$ is the characteristic function of a standard Gaussian, and $c$ is a universal constant.
\end{theorem}
If both $\delta$ and $\eta_p$ are $o(1)$, Theorem \ref{thm:almost_everywhere_clt} implies that Assumption \ref{assump:clt} is satisfied for any compact subset $\cS'_p \subseteq \cS_p$. This suggests that the norm concentration property of \eqref{eq:norm_concentration} is a convenient proxy for one-dimensional CLTs. However, the proof of this theorem uses isoperimetric inequalities, and is thus non-constructive; as a result, characterizing precisely the set $\cS_p$ remains an open and challenging mathematical problem.

\paragraph{Concentrated vectors} In \cite{seddik_2020_random}, the authors consider the concept of \emph{concentrated} random variables, as defined in \cite{ledoux_2001_concentration}:
\begin{definition}\label{def:concentrated}
Let $\bm x\in \dR^p$ be a random vector. $\bm x$ is called (exponentially) concentrated if there exists two constants $C, c$ such that for any 1-Lipschitz function $f: \dR^p \to \dR$, we have
\[ \Pb{\left|f(\bm x) - \E{f(\bm x)} \right|   \geq t} \leq C e^{-ct^2}.\]
\end{definition}
Since the norm function is $1$-Lipschitz, it can be shown that any concentrated isotropic vector $\bm x$ satisfies \eqref{eq:norm_concentration}, with
\[ \eta_p \propto \left(\frac{\log(p)}{p}\right)^{1/2} \]
The converse is obviously not true; an exponential random vector still has $\eta_p \to 0$, but is not concentrated. However, even if it is stronger that \eqref{eq:norm_concentration}, the concept of concentrated vectors has two important properties:
\begin{enumerate}
    \item a standard Gaussian vector $\bm x \sim \cN(\bm 0, \bm I_p)$ satisfies Definition \ref{def:concentrated} with constants $C, c$ independent from $p$,
    \item if $\bm x \in \dR^p$ is a concentrated vector with constants $C, c$ and $\Psi: \dR^p \to \dR^{q}$ is an $L$-Lipschitz function, then $\Psi(\bm x)$ is also a concentrated vector, with constants only depending on $c, C$ and $L$.
\end{enumerate}

\paragraph{Towards real-world datasets} The real-world data considered in machine learning is often composed of very high-dimensional inputs, corresponding to $p \gg 1$ in our setting. However, it is generally accepted that this data actually lies on a low-dimensional manifold of dimension $d_0$: this is the idea behind many dimensionality reduction techniques, from PCA \citep{pearson_1901_lines} to autoencoders \citep{kramer_1991_nonlinear}. Another, more recent line of work (see e.g. \cite{facco2017estimating}) studies the estimation of the latent dimension $d_0$; results for the MNIST dataset ($p=784$) yield $d_0 \approx 15$, while CIFAR-10 ($p=3072$) has estimated intrisic dimension $d_0\approx 35$ \citep{spigler2019asymptotic}.

Following this heuristic, the most widely used method to model realistic data is to learn a map $f: \dR^{d_0} \to \dR^p$, usually through a deep neural network, and then generate the $x_i$ according to
\begin{equation}
    \bm x = f(\bm z) \quad \text{with} \quad \bm z\sim \cN(\bm 0, \bm I_{d_0})
\end{equation} 
Examples of functions $f$ include GANs \citep{goodfellow2014generative}, variational auto-encoders \citep{kingma2013auto}, or normalizing flows \citep{rezende_2015_variational}. This ansatz has been studied theoretically, and the results compared with real-world datasets, in \cite{goldt2019modelling, loureiro2021learning}; the results indicate significant agreement between generated inputs and actual data.

Finally, we argue that for a large class of generative networks, the learned function $f$ is actually Lipschitz, with a bounded constant. This is even often a design choice; indeed, theoretical results such as \cite{bartlett_2017_spectrally} imply that a smaller Lipschitz constant improve the generalization capabilities of a network, or its numerical stability \citep{behrmann_2021_understanding}. As a result, regularizations aimed at controlling the Lipschitz properties of a network are a common occurence; see e.g. \cite{miyato_2018_spectral} for the spectral regularization of GANs. This indicates that concentrated vectors are indeed a good approximation for real-world data.
